# Supplementary material for: GPT-4V in Wonderland: Large Multimodal Models for Zero-Shot Smartphone GUI Navigation
Source: arXiv:2311.07562 source file (2023-11-13)
Supplement: Supplementary file 1 [file A-placeholder.tex]

\section{Appendix}
\subsection{Prompt templates}
\label{sec:appendix}
